# Supplementary material for: Translating the Unseen? Yoruba-English MT in Low-Resource, Morphologically-Unmarked Settings
Source: arXiv:2103.04225 source file (2021-04-06)
Supplement: Supplementary file 1 [file appendix.tex]

\clearpage
\clearpage

\twocolumn[{

}]
\appendixpage
\onecolumn
\addappheadtotoc
\counterwithin{figure}{section}
\counterwithin{table}{section}

\section{Model Errors}
\begin{table*}[h!]
\small
\begin{center}
\begin{tabular}{p{3cm} p{13cm}}
\hline
 \thead{\textbf{Output}} & \thead{\textbf{Sentence}} \\
 \hline 
 \endfirsthead
 \thead{\textbf{Missing word}} \\
 \hline
 Y{o}r\`{u}b\'{a} Source & n\'{i}tor\'{i} \`{i}d\'{i}  \`{e}y\'{i} \textsubdot{o}l\textsubdot{\'{o}}run r\'{a}n ohun t\'{o} \'{n} \textsubdot{s}i\textsubdot{s}\textsubdot{\'{e}} \`{i}\textsubdot{s}\`{i}n\`{a} s\'{i} w\textsubdot{o}n k\'{i} w\textsubdot{o}n l\`{e} gba \textbf{\`{e}k\`{e}} gb\textsubdot{\'{o}}  \\ 
 English Gold & for this reason god sends them a powerful delusion so that they will believe \textbf{the lie} \\ 
 SMT output & for this reason them powerful god sends delusion we believe that they will bear \textbf{the lie} \\ 
 BiLSTM output & therefore , god sent what the work of the work that they might believe ,  \\ 
 Transformer output & therefore , this is why god has sent them to talk about their error so that they may believe  \\ \hline \hline
  \thead{\textbf{Wrong word or spelling}} \\
 \hline
 Y{o}r\`{u}b\'{a} Source & \`{e}mi k\`{o} s\`{i} ri   \textbf{t\textsubdot{e}mpili} n\'{i}n\'{u} r\textsubdot{\`{e}} : 
 n\'{i}tor\'{i} p\'{e} ol\'{u}wa  \textsubdot{o}l\textsubdot{\'{o}}run ol\'{o}d\`{u}mar\`{e} ni t\textsubdot{e}mpili r\textsubdot{\`{e}} \`{a}ti \textsubdot{\`{o}}d\textsubdot{\'{o}} - \`{a}g\`{u}nt\`{a}n . \\ 
 English Gold & I did not see \textbf{a temple} in the city , because the Lord God Almighty and the Lamb are its temple . \\ 
 SMT output & but it did not see it the city was \textbf{temple} , because the lord god almighty are its lamb and the temple . \\ 
 BiLSTM output & and i not see \textbf{the temple} in it , for the lord the god almighty , his temple , and the lamb .,  \\ 
 Transformer output & i will not see \textbf{his temple} in the temple of the sovereign lord , for the god of his temple was lamb , and the lamb was lamb   \\ \hline \hline
 \thead{\textbf{Grammaticality}} \\
 \hline
 Y{o}r\`{u}b\'{a} Source & n\'{i}gb\`{a} n\'{a}\`{a} ol\'{u}wa \textsubdot{s}\'{i} oj\'{u} balaamu , \'{o} s\`{i} r\'{i} \'{a}ng\textsubdot{\'{e}}l\`{i} ol\'{u}wa t\'{i} \'{o} d\'{u}r\'{o} n\'{i} oj\'{u} \textsubdot{\`{o}}n\`{a} p\textsubdot{\`{e}}l\'{u} id\'{a} r\textsubdot{\`{e}} t\'{i} \'{o} f\`{a}y\textsubdot{o} . \'{o} s\`{i} t\textsubdot{e} or\'{i} r\textsubdot{\`{e}} ba . \\ 
 English Gold & then the LORD opened Balaam's eyes , and he saw the angel of the LORD standing in the road with his sword drawn . so he bowed low and fell facedown . \\ 
 
 SMT output & then balaam opened . the lord's eyes , property and saw the angel of the lord standing in turn the road with drawn sword . tied his property bowed low and fell facedown . \\ 
 BiLSTM output & then the lord opened the servant of balaam and saw the angel of the lord who preceded him with his sword , and he bowed down to her .  \\ 
 Transformer output & then the lord opened the eyes of balaam , saw the angel standing in the eyes of the lord , standing on his face . he tore his face down on his head . \\ \hline \hline
  \thead{\textbf{Wrong word or phrase order}} \\
 \hline
  Y{o}r\`{u}b\'{a} Source & et\'{i} t\'{i}ran  \'{n} gb\textsubdot{\'{o}} \`{a}ti oj\'{u} t\'{i} \'{o} \'{n} r\'{i}ran ol\'{u}wa ni \'{o} d\'{a} m\'{e}j\`{e}\`{e}j\`{i} . \\ 
 English Gold & ears that hear and eyes that see- the LORD has made them both . \\ 
 SMT output & and ears that hear \textbf{see- eyes} that the lord has made them both . \\ 
 BiLSTM output & the ear who hears the face and the eyes of the lord .  \\ 
 Transformer output & the ears of the eyes and the eyes of the lord jesus who looked at both . \\ \hline 

\end{tabular}
\end{center}
\caption{Example of errors for the three models under each error category we described. The English Gold is the NIV translation for the Y{o}r\`{u}b\'{a} Source }\label{tab:error-analysis}
\end{table*}
